# Supplementary material for: Interactive Dimensionality Reduction for Comparative Analysis
Source: arXiv:2106.15481 source file (2021-10-27)
Supplement: Supplementary file 2 [file mnist1.tex]

% [inline block 0: 1 envs, 98194 chars -> data_tex | \begin{tabular}{lrrrrrrrr} \toprule...]
