# Supplementary material for: Interactive Dimensionality Reduction for Comparative Analysis
Source: arXiv:2106.15481 source file (2021-10-27)
Supplement: Supplementary file 5 [file ppic1.tex]

\begin{tabular}{lrrrrrrrr}
\toprule
{} &   PCA (x) &   PCA (y) &   LDA (x) &  LDA (y) &  cPCA (x) &  cPCA (y) &  ULCA (x) &  ULCA (y) \\
\midrule
q1   & -0.262499 & -0.029540 & -0.135952 &      0.0 &  0.689553 &  0.162083 & -0.344023 & -0.050108 \\
q7   &  0.061919 & -0.412986 & -0.097428 &      0.0 & -0.013778 &  0.139085 &  0.036106 & -0.019798 \\
q13  & -0.064540 & -0.360961 &  0.018720 &      0.0 & -0.161281 &  0.015959 & -0.020793 & -0.004293 \\
q18  & -0.013561 & -0.076335 & -0.069628 &      0.0 &  0.095442 & -0.008482 &  0.001541 &  0.020085 \\
q19  & -0.078830 & -0.045852 & -0.178542 &      0.0 & -0.006679 &  0.055236 &  0.057741 & -0.037453 \\
q20  &  0.301285 & -0.056628 &  0.374915 &      0.0 &  0.168030 &  0.427085 &  0.183248 & -0.504519 \\
q21  &  0.172963 &  0.011879 & -0.009094 &      0.0 &  0.068641 &  0.063169 &  0.046290 & -0.021867 \\
q21a &  0.292849 & -0.010057 &  0.352594 &      0.0 &  0.119974 &  0.193656 &  0.051198 &  0.651416 \\
q22  &  0.264119 & -0.079989 &  0.052627 &      0.0 &  0.117895 &  0.118933 & -0.111115 &  0.027239 \\
q23  &  0.202948 & -0.056151 &  0.009101 &      0.0 & -0.014212 &  0.194740 &  0.123681 & -0.181099 \\
q24  & -0.242087 & -0.080452 & -0.101145 &      0.0 &  0.093145 & -0.157120 &  0.064125 &  0.459837 \\
q25  & -0.238140 & -0.035276 &  0.018476 &      0.0 &  0.223884 & -0.015996 & -0.000025 &  0.047087 \\
q26  &  0.282375 & -0.043620 & -0.144249 &      0.0 &  0.293312 &  0.204617 & -0.006155 &  0.053229 \\
q27  & -0.259116 &  0.005183 & -0.087271 &      0.0 & -0.277763 &  0.489935 &  0.053455 & -0.122329 \\
q28  & -0.253654 & -0.045732 & -0.318113 &      0.0 & -0.259232 &  0.232197 &  0.147868 &  0.002127 \\
q29  & -0.264244 & -0.044850 & -0.033479 &      0.0 & -0.133985 &  0.002701 & -0.127783 & -0.110617 \\
q30  & -0.244617 & -0.073278 & -0.328858 &      0.0 & -0.018518 &  0.143548 &  0.851559 &  0.024652 \\
q31  &  0.265555 & -0.000986 &  0.334397 &      0.0 & -0.123369 & -0.229083 & -0.161481 & -0.046006 \\
q33  & -0.257920 & -0.076160 & -0.274269 &      0.0 & -0.038854 &  0.320887 & -0.040543 & -0.118824 \\
q34  &  0.017638 & -0.452132 & -0.002937 &      0.0 & -0.157850 &  0.156949 &  0.028108 &  0.094607 \\
q36  &  0.028359 & -0.385510 &  0.041148 &      0.0 & -0.063469 &  0.196644 & -0.047058 & -0.067060 \\
q37a & -0.003487 & -0.078765 &  0.013674 &      0.0 &  0.047617 &  0.169870 & -0.012261 & -0.010002 \\
d3a  &  0.023643 & -0.250583 & -0.011744 &      0.0 &  0.125461 & -0.001833 & -0.000281 &  0.027467 \\
d6   & -0.000859 & -0.114435 & -0.029078 &      0.0 & -0.114432 &  0.109959 &  0.050348 &  0.017560 \\
d7   & -0.033413 & -0.259972 &  0.123900 &      0.0 & -0.112893 &  0.159850 &  0.067566 & -0.047822 \\
d9a  &  0.043446 & -0.120803 &  0.038419 &      0.0 & -0.116516 &  0.081919 &  0.018063 & -0.056948 \\
d1a  &  0.037022 & -0.367580 &  0.024154 &      0.0 &  0.130929 & -0.041311 & -0.043981 &  0.041030 \\
\bottomrule
\end{tabular}
