# Supplementary material for: Interactive Dimensionality Reduction for Comparative Analysis
Source: arXiv:2106.15481 source file (2021-10-27)
Supplement: Supplementary file 6 [file ppic2.tex]

\begin{tabular}{lrrrrrrrr}
\toprule
{} &   PCA (x) &   PCA (y) &  LDA (x) &  LDA (y) &  cPCA (x) &  cPCA (y) &  ULCA (x) &  ULCA (y) \\
\midrule
q1   & -0.272006 & -0.025406 &        0 &        0 &  0.472050 &  0.373206 &  0.558180 &  0.159270 \\
q7   &  0.051561 & -0.415685 &        0 &        0 & -0.085978 & -0.005874 & -0.183562 &  0.071507 \\
q13  & -0.068367 & -0.347333 &        0 &        0 & -0.065163 &  0.004781 &  0.015901 & -0.270734 \\
q18  & -0.015867 & -0.121445 &        0 &        0 &  0.001138 & -0.024359 & -0.015735 & -0.003108 \\
q19  & -0.086224 & -0.067838 &        0 &        0 &  0.055548 &  0.118862 &  0.093673 & -0.043103 \\
q20  &  0.307895 & -0.044009 &        0 &        0 &  0.199424 &  0.494824 & -0.132921 &  0.339701 \\
q21  &  0.180770 &  0.015282 &        0 &        0 &  0.032325 &  0.045913 &  0.086195 & -0.030779 \\
q21a &  0.296603 &  0.011459 &        0 &        0 &  0.197613 & -0.489857 & -0.222388 &  0.412679 \\
q22  &  0.270156 & -0.062986 &        0 &        0 &  0.194321 & -0.017552 &  0.118428 &  0.050037 \\
q23  &  0.203250 & -0.043077 &        0 &        0 & -0.073007 &  0.009687 & -0.157588 &  0.100453 \\
q24  & -0.253813 & -0.053852 &        0 &        0 &  0.271304 & -0.120468 &  0.317152 &  0.080041 \\
q25  & -0.252807 & -0.008591 &        0 &        0 &  0.386441 & -0.096710 & -0.013817 &  0.433229 \\
q26  &  0.288913 & -0.046929 &        0 &        0 &  0.373558 & -0.115602 &  0.225641 &  0.314264 \\
q27  & -0.266678 &  0.006934 &        0 &        0 & -0.153651 &  0.278042 &  0.069138 & -0.276877 \\
q28  & -0.261923 & -0.055755 &        0 &        0 & -0.340273 &  0.052775 & -0.192458 & -0.321027 \\
q29  & -0.273050 & -0.041173 &        0 &        0 & -0.090726 & -0.413597 & -0.381342 & -0.012470 \\
q31  &  0.276355 & -0.021581 &        0 &        0 & -0.258279 &  0.108430 &  0.000249 & -0.175618 \\
q33  & -0.270587 & -0.074903 &        0 &        0 &  0.163379 & -0.122102 &  0.000337 &  0.086607 \\
q34  &  0.013855 & -0.446806 &        0 &        0 &  0.118189 & -0.073985 &  0.152876 &  0.019129 \\
q36  &  0.024034 & -0.365329 &        0 &        0 &  0.005342 & -0.101658 & -0.247427 &  0.155303 \\
q37a & -0.002479 & -0.094320 &        0 &        0 &  0.032020 &  0.027129 &  0.095491 & -0.030879 \\
d3a  &  0.013835 & -0.259995 &        0 &        0 &  0.010438 &  0.113828 &  0.159899 & -0.062622 \\
d6   & -0.010729 & -0.079336 &        0 &        0 & -0.056727 & -0.018921 & -0.046021 & -0.178001 \\
d7   & -0.039018 & -0.279497 &        0 &        0 & -0.035465 &  0.047200 & -0.087423 &  0.133693 \\
d9a  &  0.043838 & -0.115847 &        0 &        0 & -0.058634 & -0.100970 & -0.192951 &  0.056562 \\
d1a  &  0.032435 & -0.393590 &        0 &        0 &  0.113705 &  0.035856 &  0.163867 &  0.043843 \\
\bottomrule
\end{tabular}
