# Supplementary material for: Interactive Dimensionality Reduction for Comparative Analysis
Source: arXiv:2106.15481 source file (2021-10-27)
Supplement: Supplementary file 7 [file ppic3.tex]

\begin{tabular}{lrrrrrrrr}
\toprule
{} &   PCA (x) &   PCA (y) &   LDA (x) &  LDA (y) &  cPCA (x) &  cPCA (y) &  ULCA (x) &  ULCA (y) \\
\midrule
q1   & -0.272006 & -0.025406 & -0.181956 &      0.0 &  0.472050 &  0.373206 & -0.191644 & -0.124360 \\
q7   &  0.051561 & -0.415685 & -0.113320 &      0.0 & -0.085978 & -0.005874 &  0.107413 &  0.004499 \\
q13  & -0.068367 & -0.347333 & -0.011961 &      0.0 & -0.065163 &  0.004781 & -0.075113 & -0.083833 \\
q18  & -0.015867 & -0.121445 & -0.059593 &      0.0 &  0.001138 & -0.024359 & -0.062652 & -0.075154 \\
q19  & -0.086224 & -0.067838 & -0.165659 &      0.0 &  0.055548 &  0.118862 & -0.071863 & -0.086774 \\
q20  &  0.307895 & -0.044009 &  0.449496 &      0.0 &  0.199424 &  0.494824 &  0.790036 & -0.142629 \\
q21  &  0.180770 &  0.015282 &  0.003009 &      0.0 &  0.032325 &  0.045913 &  0.002213 &  0.031159 \\
q21a &  0.296603 &  0.011459 &  0.346843 &      0.0 &  0.197613 & -0.489857 &  0.023907 &  0.676308 \\
q22  &  0.270156 & -0.062986 &  0.047464 &      0.0 &  0.194321 & -0.017552 &  0.032788 &  0.171582 \\
q23  &  0.203250 & -0.043077 &  0.022052 &      0.0 & -0.073007 &  0.009687 &  0.169506 &  0.060299 \\
q24  & -0.253813 & -0.053852 & -0.159578 &      0.0 &  0.271304 & -0.120468 & -0.347739 &  0.057961 \\
q25  & -0.252807 & -0.008591 &  0.014950 &      0.0 &  0.386441 & -0.096710 &  0.028889 &  0.156015 \\
q26  &  0.288913 & -0.046929 & -0.113532 &      0.0 &  0.373558 & -0.115602 & -0.144949 &  0.331211 \\
q27  & -0.266678 &  0.006934 & -0.087042 &      0.0 & -0.153651 &  0.278042 &  0.016656 & -0.235233 \\
q28  & -0.261923 & -0.055755 & -0.341739 &      0.0 & -0.340273 &  0.052775 & -0.120233 & -0.436055 \\
q29  & -0.273050 & -0.041173 & -0.080050 &      0.0 & -0.090726 & -0.413597 & -0.046404 & -0.123246 \\
q31  &  0.276355 & -0.021581 &  0.311197 &      0.0 & -0.258279 &  0.108430 &  0.180075 &  0.136549 \\
q33  & -0.270587 & -0.074903 & -0.271110 &      0.0 &  0.163379 & -0.122102 & -0.182615 & -0.109055 \\
q34  &  0.013855 & -0.446806 &  0.003489 &      0.0 &  0.118189 & -0.073985 & -0.134511 &  0.087867 \\
q36  &  0.024034 & -0.365329 &  0.035556 &      0.0 &  0.005342 & -0.101658 &  0.086948 &  0.047533 \\
q37a & -0.002479 & -0.094320 &  0.014897 &      0.0 &  0.032020 &  0.027129 & -0.044884 &  0.000106 \\
d3a  &  0.013835 & -0.259995 & -0.020982 &      0.0 &  0.010438 &  0.113828 & -0.011600 &  0.075408 \\
d6   & -0.010729 & -0.079336 & -0.040659 &      0.0 & -0.056727 & -0.018921 &  0.027291 &  0.061168 \\
d7   & -0.039018 & -0.279497 &  0.137705 &      0.0 & -0.035465 &  0.047200 &  0.149902 &  0.052898 \\
d9a  &  0.043838 & -0.115847 &  0.043950 &      0.0 & -0.058634 & -0.100970 &  0.076157 &  0.040297 \\
d1a  &  0.032435 & -0.393590 &  0.021741 &      0.0 &  0.113705 &  0.035856 & -0.014708 &  0.009417 \\
\bottomrule
\end{tabular}
