# Supplementary material for: Interactive Dimensionality Reduction for Comparative Analysis
Source: arXiv:2106.15481 source file (2021-10-27)
Supplement: Supplementary file 8 [file wine1.tex]

\begin{tabular}{lrrrrrrrr}
\toprule
{} &   PCA (x) &   PCA (y) &   LDA (x) &   LDA (y) &  cPCA (x) &  cPCA (y) &  ULCA (x) &  ULCA (y) \\
\midrule
alcohol              &  0.144329 & -0.483652 & -0.326569 &  0.705754 &         0 &         0 &  0.047908 &  0.222532 \\
malic\_acid           & -0.245188 & -0.224931 &  0.184094 &  0.340194 &         0 &         0 & -0.119098 & -0.001570 \\
ash                  & -0.002051 & -0.316069 & -0.100969 &  0.641759 &         0 &         0 & -0.068764 &  0.373212 \\
alcalinity\_of\_ash    & -0.239320 &  0.010591 &  0.515503 & -0.487473 &         0 &         0 & -0.140328 & -0.391263 \\
magnesium            &  0.141992 & -0.299634 & -0.030813 & -0.006591 &         0 &         0 &  0.020823 & -0.065924 \\
total\_phenols        &  0.394661 & -0.065040 &  0.385720 & -0.020104 &         0 &         0 & -0.052743 &  0.232090 \\
flavanoids           &  0.422934 &  0.003360 & -1.654628 & -0.490054 &         0 &         0 &  0.780194 & -0.385695 \\
nonflavanoid\_phenols & -0.298533 & -0.028779 & -0.185636 & -0.202407 &         0 &         0 &  0.062533 & -0.143723 \\
proanthocyanins      &  0.313429 & -0.039302 &  0.076533 & -0.175270 &         0 &         0 &  0.016385 &  0.054407 \\
color\_intensity      & -0.088617 & -0.529996 &  0.820805 &  0.585410 &         0 &         0 & -0.344212 & -0.115462 \\
hue                  &  0.296715 &  0.279235 & -0.186454 & -0.345456 &         0 &         0 &  0.227938 & -0.007595 \\
od280/od315          &  0.376167 &  0.164496 & -0.819544 &  0.036238 &         0 &         0 &  0.362277 &  0.386084 \\
proline              &  0.286752 & -0.364903 & -0.845097 &  0.895899 &         0 &         0 &  0.203277 &  0.514844 \\
\bottomrule
\end{tabular}
