# Supplementary material for: Interactive Dimensionality Reduction for Comparative Analysis
Source: arXiv:2106.15481 source file (2021-10-27)
Supplement: Supplementary file 9 [file wine2.tex]

\begin{tabular}{lrrrrrrrr}
\toprule
{} &   PCA (x) &   PCA (y) &   LDA (x) &  LDA (y) &  cPCA (x) &  cPCA (y) &  ULCA (x) &  ULCA (y) \\
\midrule
alcohol              &  0.144329 & -0.483652 & -0.721476 &      0.0 &         0 &         0 &  0.233373 &  0.437619 \\
malic\_acid           & -0.245188 & -0.224931 & -0.104383 &      0.0 &         0 &         0 &  0.004880 & -0.052372 \\
ash                  & -0.002051 & -0.316069 & -0.516378 &      0.0 &         0 &         0 &  0.012357 &  0.282481 \\
alcalinity\_of\_ash    & -0.239320 &  0.010591 &  0.704967 &      0.0 &         0 &         0 & -0.093801 & -0.512145 \\
magnesium            &  0.141992 & -0.299634 & -0.017396 &      0.0 &         0 &         0 & -0.090407 &  0.200818 \\
total\_phenols        &  0.394661 & -0.065040 &  0.288819 &      0.0 &         0 &         0 &  0.125364 &  0.175940 \\
flavanoids           &  0.422934 &  0.003360 & -0.839866 &      0.0 &         0 &         0 &  0.446139 & -0.047882 \\
nonflavanoid\_phenols & -0.298533 & -0.028779 &  0.007867 &      0.0 &         0 &         0 & -0.102017 &  0.027326 \\
proanthocyanins      &  0.313429 & -0.039302 &  0.175919 &      0.0 &         0 &         0 &  0.051957 &  0.027711 \\
color\_intensity      & -0.088617 & -0.529996 &  0.179579 &      0.0 &         0 &         0 &  0.097398 &  0.017415 \\
hue                  &  0.296715 &  0.279235 &  0.106346 &      0.0 &         0 &         0 &  0.141806 &  0.005798 \\
od280/od315          &  0.376167 &  0.164496 & -0.609172 &      0.0 &         0 &         0 & -0.152601 &  0.620854 \\
proline              &  0.286752 & -0.364903 & -1.222698 &      0.0 &         0 &         0 &  0.804762 & -0.052649 \\
\bottomrule
\end{tabular}
