# Supplementary material for: Interactive Dimensionality Reduction for Comparative Analysis
Source: arXiv:2106.15481 source file (2021-10-27)
Supplement: Supplementary file 10 [file wine3.tex]

\begin{tabular}{lrrrrrrrr}
\toprule
{} &   PCA (x) &   PCA (y) &  LDA (x) &  LDA (y) &  cPCA (x) &  cPCA (y) &  ULCA (x) &  ULCA (y) \\
\midrule
alcohol              &  0.144329 & -0.483652 &        0 &        0 &  0.018234 & -0.473961 & -0.144189 &  0.073715 \\
malic\_acid           & -0.245188 & -0.224931 &        0 &        0 & -0.004813 &  0.085529 &  0.092141 & -0.057192 \\
ash                  & -0.002051 & -0.316069 &        0 &        0 &  0.027183 & -0.238400 & -0.003362 &  0.066421 \\
alcalinity\_of\_ash    & -0.239320 &  0.010591 &        0 &        0 &  0.012851 & -0.045151 &  0.049720 &  0.003406 \\
magnesium            &  0.141992 & -0.299634 &        0 &        0 & -0.163372 &  0.028401 &  0.008755 & -0.088388 \\
total\_phenols        &  0.394661 & -0.065040 &        0 &        0 &  0.442786 &  0.010927 & -0.243510 &  0.511967 \\
flavanoids           &  0.422934 &  0.003360 &        0 &        0 & -0.742596 &  0.071961 & -0.100889 & -0.811436 \\
nonflavanoid\_phenols & -0.298533 & -0.028779 &        0 &        0 &  0.257193 &  0.216337 & -0.077980 &  0.128603 \\
proanthocyanins      &  0.313429 & -0.039302 &        0 &        0 &  0.192331 & -0.135110 &  0.012373 &  0.163924 \\
color\_intensity      & -0.088617 & -0.529996 &        0 &        0 &  0.232810 & -0.238384 &  0.903389 &  0.061729 \\
hue                  &  0.296715 &  0.279235 &        0 &        0 &  0.026516 &  0.005303 &  0.089583 & -0.026993 \\
od280/od315          &  0.376167 &  0.164496 &        0 &        0 &  0.250281 &  0.197020 &  0.127810 &  0.102718 \\
proline              &  0.286752 & -0.364903 &        0 &        0 &  0.062119 &  0.736438 & -0.227985 & -0.004630 \\
\bottomrule
\end{tabular}
